# Supplementary material for: Efficient Contraction of Large Tensor Networks for Weighted Model Counting through Graph Decompositions
Source: arXiv:1908.04381 source file (2020-04-27)
Supplement: Supplementary file 1 [file appendix_definitions.tex]

\section{Additional Definitions and Notations}
For convenience, we also state here the complete definitions of the graph  decompositions we require: carving decompositions and tree decompositions. Both decompose the graph into an \emph{unrooted binary tree}, which is a tree where
every vertex has degree one or three.  First, we describe carving decompositions \cite{ST94}:
\begin{definition}[Carving Decomposition]
\label{def:carving}
	Let $G$ be a graph. A \emph{carving decomposition} of $G$ is an unrooted binary tree $T$ whose leaves are the vertices of $G$, i.e. $\Lv{T} = \V{G}$. 
	
    For every arc $a$ of $T$, deleting $a$ from $T$ yields exactly two trees, whose leaves define a partition of the vertices of $G$. Let $C_a \subseteq \V{G}$ be an arbitrary element of this partition. The \emph{width} of $T$, denoted $width_c(T)$, is the maximum number of edges in $G$ between $C_a$ and $\V{G} \setminus C_a$ for all $a \in \E{T}$, i.e.,
	$$width_c(T) = \max_{a \in \E{T}} \left| \vinc{G}{C_a} \cap \vinc{G}{\V{G} \setminus C_a} \right|.$$
    The width of a carving decomposition $T$ with no edges is 0.
\end{definition}

In Definition \ref{def:carving}, $\vinc{G}{V}$ refers to the set of edges of $G$ incident to some vertex in $V \subseteq \V{G}$. The \emph{carving width} of a graph $G$ is the minimum width across all carving decompositions of $G$.

Next, we define tree decompositions \cite{RS91}:
\begin{definition}[Tree Decomposition]
	Let $G$ be a graph. A \emph{tree decomposition} of $G$ is an unrooted binary tree $T$ together with a labeling function $\chi : \V{T} \rightarrow 2^{\V{G}}$ that satisfies the following three properties:
	\begin{enumerate}
		\item Every vertex of $G$ is contained in the label of some node of $T$. That is, $\V{G} = \bigcup_{n \in \V{T}} \chi(n)$.
		\item For every edge $e \in \E{G}$, there is a node $n \in \V{T}$ whose label is a superset of $\einc{G}{e}$, i.e. $\einc{G}{e} \subseteq \chi(n)$.
		\item If $n$ and $o$ are nodes in $T$, and $p$ is a node on the path from $n$ to $o$, then $\chi(n) \cap \chi(o) \subseteq \chi(p)$.
	\end{enumerate}
	The \emph{width} of a tree decomposition, denoted $width_t(T, \chi)$, is the maximum size (minus 1) of the label of every node, i.e.,
	$$width_t(T, \chi) = \max_{n \in \V{T}} | \chi(n) | - 1.$$
\end{definition}
The \emph{treewidth} of a graph $G$ is the minimum width across all tree decompositions of $G$. The treewidth of a tree is $1$.
